# Supplementary material for: Differentially private significance tests for regression coefficients
Source: arXiv:1705.09561 ancillary file (2018-06-11)
Supplement: Supplementary file 1 [file supplementary_material.pdf]

# Supplementary Material: Differentially Private Significance Tests for Regression Coefficients

Andrés F. Barrientos, Jerome P. Reiter, Ashwin Machanavajjhala, Yan Chen *

This document presents supplementary material to the main text of the paper. In Section 1, we include a graphical representation of the upper bound provided in Theorem 2 of the main text, as well as the proof of Theorem 2. In Section 2, we include additional plots associated with Sections 5.1 and 5.2 of the main text when $\epsilon = \infty$, and with Section 5.3 when the maximum of the matching probabilities is taken over $(M, a)$ for fixed $\epsilon$. In Section 3, we present the p-values and signs for the coefficients in the examples considered in Section 6 of the paper.

# 1 Graphical representation and proof of Theorem 2

In this section, we first present a graphical representation of the upper bound in Theorem 2 of the paper. We referred to this figure at the end of Section 4.2 of the main text. Then, we provide the proof of this theorem.

## 1.1 Upper bound for the asymptotic type II error probability

Figure 1 shows how the upper bound for $\lim_{n\to\infty} E_{H_1}\left\{\mathbb{T}^{t,\epsilon}(\mathcal{P})\,|\mathbf{X}_{\boldsymbol{D}}, \mathcal{R}\right\}$ behaves for different values of $(\alpha, M, a, \epsilon)$. These plots are comparable to those in Figure 2 in the main text. We conclude that Theorem 2 can provide sharp bounds, particularly when $a > 2$. For $1 \leq a \leq 2$ and some values of $M$, the bound is a moderately less precise, but still valid, bound for $\lim_{n\to\infty} E_{H_1}\left\{\mathbb{T}^{t,\epsilon}(\mathcal{P})\,|\mathbf{X}_{\boldsymbol{D}}, \mathcal{R}\right\}$. Although we view $\epsilon$ as fixed for privacy purposes, we can see that the derived bound decreases as $\epsilon$ increases, holding $(\alpha, M, a)$ constant.

*Andrés F. Barrientos is Postdoctoral Associate, Department of Statistical Science, Duke University, Durham, NC 27708 (email: afb26@stat.duke.edu); Jerome Reiter is Professor, Department of Statistical Science, Duke University, Durham, NC 27708 (jerry@stat.duke.edu); Ashwin Machanavajjhala is Assistant Professor, Department of Computer Science, Duke University, Durham, NC 27708 (ashwin@cs.duke.edu); and, Yan Chen is Graduate Student, Department of Computer Science, Duke University, Durham, NC 27708 (yanchen@cs.duke.edu).

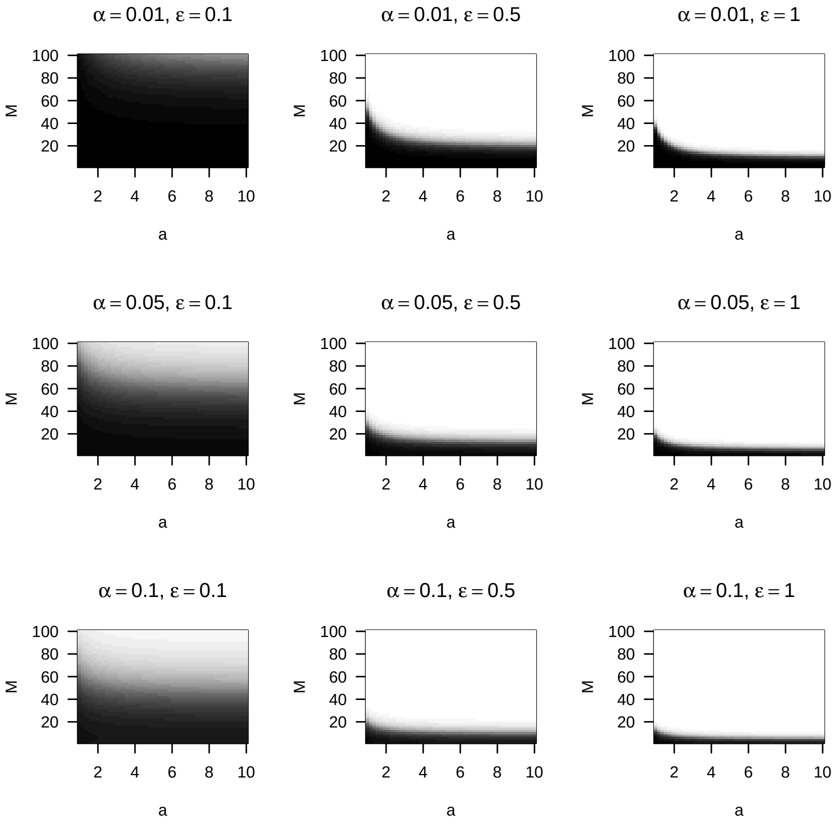


Figure 1: Upper bound for the asymptotic probability of type II error associated with the test $\mathbb{T}^{t,\epsilon}(\mathcal{P})$ for different values of $(\alpha, a, M, \epsilon)$. Within any panel and combination $(M, a)$, black represents $\lim_{n\to\infty} E_{H_1}\{\mathbb{T}^{t,\epsilon}(\mathcal{P})\,|\mathbf{X}_{\boldsymbol{D}}, \mathcal{R}\} = 1$ and white represents $\lim_{n\to\infty} E_{H_1}\{\mathbb{T}^{t,\epsilon}(\mathcal{P})\,|\mathbf{X}_{\boldsymbol{D}}, \mathcal{R}\} = 0$, with lighter grays as the loss function approaches 0.

## 1.2 Proof of Theorem 2

We assume without loss of generality that $\beta_j > 0$. Recall that we do not have an analytical expression for $r$, where $r$ is the $(1-\alpha/2)$th percentile of $\bar{T}^{t,R}(\mathcal{P}) + \eta$ and $\eta \sim \text{Lap}(2a/\sqrt{M}\epsilon)$. The lack of an analytical expression for $r$ leads us to find a upper bound for the type II error by using an upper bound for $r$. We determine an upper bound for $r$ by noticing that the $(1-\alpha/2)$th percentile of $\bar{T}^{t,R}(\mathcal{P})$ is smaller than that for $W$, where $W \sim \text{Lap}(1)$. Hence, under $H_0$, one has that $r < r^*$, where $r^*$ is the $(1-\alpha/2)$th percentile of $W + \eta \sim \text{Lap}(2a/\sqrt{M}\epsilon + 1)$.

On the other hand, we can express the type II error as

$$
\begin{aligned}
E\left\{\mathbb{T}_{t,\epsilon}\,|\mathbf{X}_{\boldsymbol{D}},\mathcal{R}\right\} &= P\left\{r<\bar{T}^{t,\epsilon}(\mathcal{P})<r\,|\mathbf{X}_{\boldsymbol{D}},\mathcal{R}\right\},\\
&= P\left\{-r<\bar{T}^{t,\epsilon}(\mathcal{P})<r\left|\bar{T}^{t,R}(\mathcal{P})=\sqrt{M}a,\mathbf{X}_{\boldsymbol{D}},\mathcal{R}\right.\right\}P\left\{\bar{T}^{t,R}(\mathcal{P})=\sqrt{M}a\,|\mathbf{X}_{\boldsymbol{D}},\mathcal{R}\right\}\\
&\quad + P\left\{-r<\bar{T}^{t,\epsilon}(\mathcal{P})<r\left|\bar{T}^{t,R}(\mathcal{P})\neq\sqrt{M}a,\mathbf{X}_{\boldsymbol{D}},\mathcal{R}\right.\right\}P\left\{\bar{T}^{t,R}(\mathcal{P})\neq\sqrt{M}a\,|\mathbf{X}_{\boldsymbol{D}},\mathcal{R}\right\}\\
&= P\left\{-r<\bar{T}^{t,\epsilon}(\mathcal{P})<r\left|\bar{T}^{t,R}(\mathcal{P})=\sqrt{M}a,\mathbf{X}_{\boldsymbol{D}},\mathcal{R}\right.\right\}\left(1-\Phi\left(a-\mu_n\right)\right)^M\\
&\quad + P\left\{-r<\bar{T}^{t,\epsilon}(\mathcal{P})<r\left|\bar{T}^{t,R}(\mathcal{P})\neq\sqrt{M}a,\mathbf{X}_{\boldsymbol{D}},\mathcal{R}\right.\right\}\left[1-\left(1-\Phi\left(a-\mu_n\right)\right)^M\right],
\end{aligned}
$$

where $\mu_n = E\{T(\boldsymbol{D}_l)|\mathbf{X}_{\boldsymbol{D}_l},\mathcal{R}\}$. Under $H_1$, one has that $\lim_{n\to\infty}\mu_n = \infty$ and, therefore, $\lim_{n\to\infty} P\left\{\bar{T}^{DP}(\mathcal{P})=\sqrt{M}a\,|\mathbf{X}_{\boldsymbol{D}},\mathcal{R}\right\}=1$. It follows that

$$
\begin{aligned}
\lim_{n\to\infty} E\left\{\mathbb{T}_{t,\epsilon}\,|\mathbf{X}_{\boldsymbol{D}},\mathcal{R}\right\} &= \lim_{n\to\infty} P\left\{-r<\bar{T}^{t,\epsilon}(\mathcal{P})<r\left|\bar{T}^{t,R}(\mathcal{P})=\sqrt{M}a,\mathbf{X}_{\boldsymbol{D}},\mathcal{R}\right.\right\},\\
&= P\left\{-r<e+\sqrt{M}a<r\right\},\\
&< P\left\{-r^*<e+\sqrt{M}a<r^*\right\}.
\end{aligned}
$$

The proof is completed by noticing that, if $r^*<\sqrt{M}a$,

$$
\begin{aligned}
P\left\{-r^*<e+\sqrt{M}a<r^*\right\} &= \frac{1}{2}\exp\left(\frac{r^*-\sqrt{M}a}{\frac{2a}{\epsilon\sqrt{M}}}\right)-\frac{1}{2}\exp\left(\frac{-r^*-\sqrt{M}a}{\frac{2a}{\epsilon\sqrt{M}}}\right)\\
&= \frac{1}{2}\left(\alpha^{-1-\epsilon\sqrt{M}/2a}-\alpha^{1+\epsilon\sqrt{M}/2a}\right)\exp\left(-\frac{\epsilon M}{2}\right).
\end{aligned}
$$

and that, if $r^*>\sqrt{M}a$,

$$
\begin{aligned}
P\left\{-r^*<e+\sqrt{M}a<r^*\right\} &= 1-\frac{1}{2}\exp\left(-\frac{r^*-\sqrt{M}a}{\frac{2a}{\epsilon\sqrt{M}}}\right)-\frac{1}{2}\exp\left(\frac{-r^*-\sqrt{M}a}{\frac{2a}{\epsilon\sqrt{M}}}\right)\\
&= 1-\frac{1}{2}\alpha^{1+\epsilon\sqrt{M}/2a}\left[\exp\left(\frac{\epsilon M}{2}\right)-\exp\left(-\frac{\epsilon M}{2}\right)\right].
\end{aligned}
$$

# 2 Additional plots for assessing the performance of $\bar{T}^{t,\epsilon}$

This section contains two additional plots associated with Section 5 of the paper. The first plot provides a graphical assessment of the inferences about significance and signs of coefficients when no noise is added to the test t-statistic. The second plot displays the maximum of the matching probabilities taken over $(M, a)$ for fixed values of $\epsilon$. The items below provide a brief description of the results.

- Figure 2 presents the results associated with the inferences about signs of coefficients. In Scenario I, the performance of $\bar{T}^{t,\epsilon}$ is quite good. In Scenario II, we identify slight differences for some combinations of $(M, a)$ and for some regression coefficients. We observe the biggest differences when $M = 100$. This arises because larger values of $M$ lead to fewer data points in $\boldsymbol{D}_l$, which can weaken the validity of assumption **A2**. We also observe that the performance of $\bar{T}^{t,\epsilon}$ is more robust to possible violations of assumption **A2** for inferring the sign than for inferring the significance. In Scenario II, $L^{sgn}_{t,\epsilon}$ seems invariant under changes in the values of $a$.

- Figure 3 displays the values of $\tilde{m}^{sig}_{t,\epsilon}(\mu_T, \epsilon)$ and $\tilde{m}^{sgn}_{t,\epsilon}(\mu_T, \epsilon)$ for different values of $\mu_T$ and $\epsilon$, where

$$\tilde{m}^{sig}_{t,\epsilon}(\mu_T, \epsilon) = \max_{M,a} P\left\{\mathbb{T}_{t,\epsilon} = \mathbb{T} | \mu_T, M, a, \epsilon, \mathbf{X}_{\boldsymbol{D}}, \mathcal{R}\right\},$$

$$\tilde{m}^{sgn}_{t,\epsilon}(\mu_T, \epsilon) = \max_{M,a} P\left\{\text{sign}(T) = \text{sign}(\bar{T}^{t,\epsilon}) | \mu_T, M, a, \epsilon, \mathbf{X}_{\boldsymbol{D}}, \mathcal{R}\right\},$$

  where each maximum is over all possible combinations of $M \in \{10, 25, 50, 75, 100\}$ and $a \in \{1, 2, \ldots, 10\}$.

  For $\tilde{m}^{sig}_{t,\epsilon}(\mu_T, \epsilon)$, we can see that under the null hypothesis, i.e., $\mu_T = 0$, values of $\tilde{m}^{sig}_{t,\epsilon}$ are near $0.91$ for Scenario I and above $0.95$ for Scenario II. In both scenarios, when $\mu_T$ is large enough, values of $\tilde{m}^{sig}_{t,\epsilon}$ are close to one. The value of $\mu_T$ at which $m^{sig}_{t,\epsilon}$ is close to one is inversely related to the value of $\epsilon$. However, for any value of $\epsilon$ and $\mu_T > 6$, $\tilde{m}^{sig}_{t,\epsilon} \approx 1$. Values of $\tilde{m}^{sig}_{t,\epsilon}$ tend to be around $0.5$ when $\mu_T \approx r$, where $r$ is the critical values associated with $\mathbb{T}$.

  For $\tilde{m}^{sgn}_{t,\epsilon}(\mu_T, \epsilon)$, as expected, in both scenarios, increases in $\mu_T$ correspond to increases in the matching probability. The rate at which $\tilde{m}^{sgn}_{t,\epsilon}$ increases as a function of $\mu_T$ depends on $\epsilon$: the larger the $\epsilon$, the faster the rate. Notice that these rates are less different in Scenario I than in Scenario II. As expected, when $\mu_T = 0$, $\tilde{m}^{sgn}_{t,\epsilon}$ reaches its minimum of $0.5$ and $0.8$ for Scenario I and II, respectively. However, when $\mu_T = 0$, matching the sign of $T$ and $\bar{T}^{t,\epsilon}$ arguably is not important for interpretations. In both scenarios, we also observe a high matching probability ($\tilde{m}^{sgn}_{t,\epsilon} > 0.9$) when $\mu_T \geq 3$ regardless the value of $\epsilon$.

  Finally, we conclude by noticing that matching probabilities for the significance and sign are higher for Scenario II than for Scenario I. This is an expected result since we expect positive correlations between $\sqrt{M}\bar{T}(\mathcal{P})$ and $T(\boldsymbol{D})$ when $\boldsymbol{D}$ is a genuine dataset–as in Scenario II. Recall that, by the results provided in Section 4 of the paper, the larger is the correlation between $\sqrt{M}\bar{T}(\mathcal{P})$ and $T(\boldsymbol{D})$, the smaller is the distance between them.

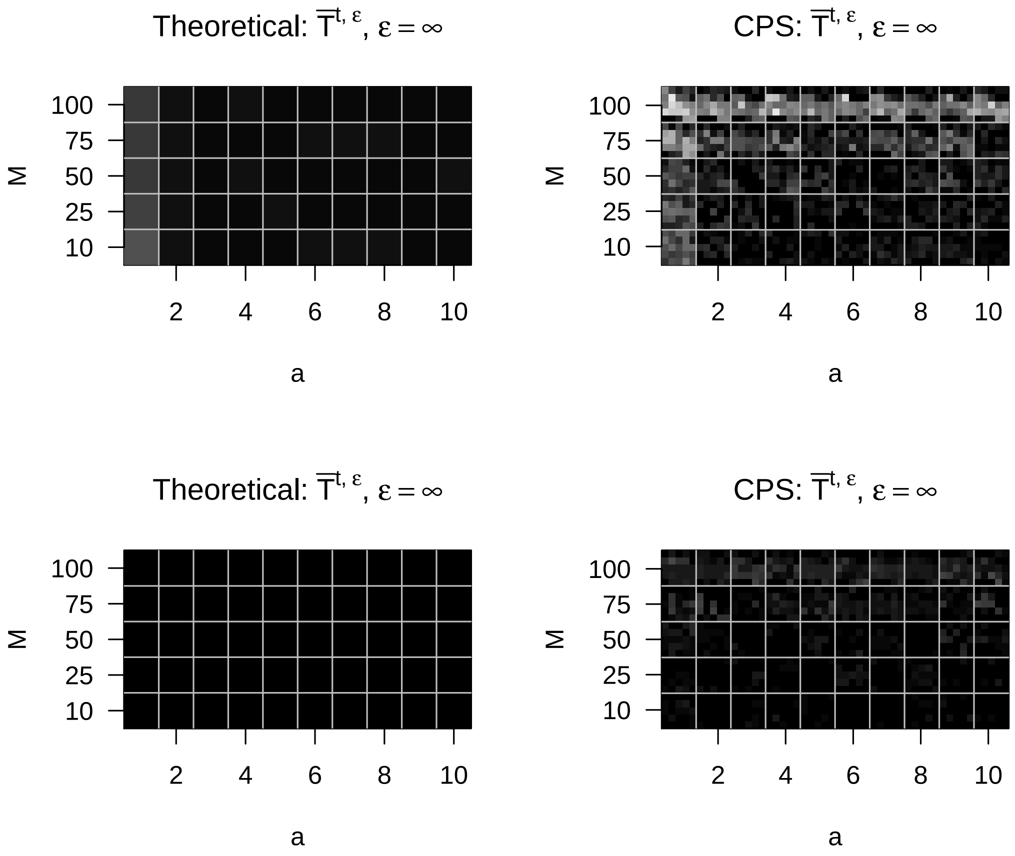


Figure 2: Values of $L_{t,\epsilon}^{sig}(M, a, \epsilon = \infty)$ and $L_{t,\epsilon}^{sgn}(M, a, \epsilon = \infty)$ at different combinations of $(M, a)$ for $(\alpha = 0.05, \lambda_0 = 0.2)$. Left and right panels show the results for $L_{t,\epsilon}^{sig}(M, a, \epsilon = \infty)$ and $L_{t,\epsilon}^{sig}(M, a, \epsilon = \infty)$, respectively. Top and bottom panels show Scenario I and II, respectively. For Scenario I, each cell represents the average of 100,000 runs at that $(M, a)$. For Scenario II, each $(M, a)$ cell comprises a $5 \times 5$ array of sub-cells representing the results for the $25$ coefficients in the CPS regression. Individual sub-cell results are averages of 1,000 runs. Within any cell or sub-cell, black represents $L_{t,\epsilon}^{k}(M, a, \infty) = 0$ and white represents $L_{t,\epsilon}^{k}(M, a, \infty) \geq 0.25$, with lighter grays as the loss function approaches 0.25 and $k \in \{sig, sgn\}$.

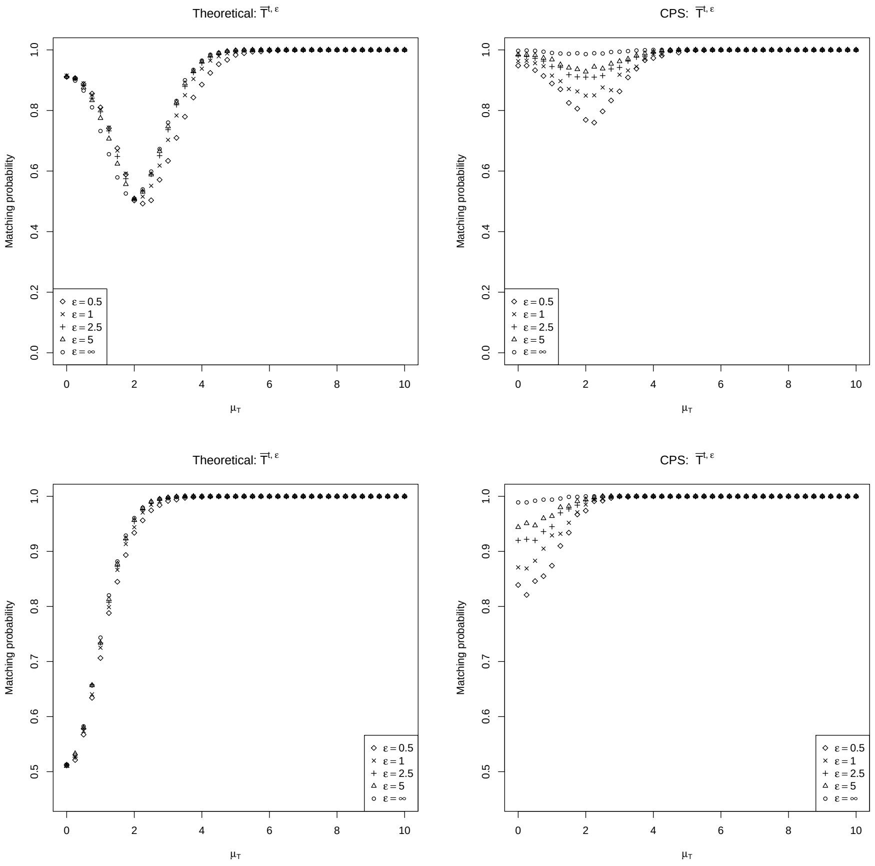


Figure 3: Values of $\tilde{m}^{sig}_{t,\epsilon}(\mu_T, \epsilon)$ and $\tilde{m}^{sgn}_{t,\epsilon}(\mu_T, \epsilon)$ at different combinations of $\mu_T$ and $\epsilon$ with $\alpha = 0.05$. Left and right panels show Scenario I and II, respectively. Top and bottom panels show the results for $\tilde{m}^{sig}_{t,\epsilon}(\mu_T, \epsilon)$ and $\tilde{m}^{sgn}_{t,\epsilon}(\mu_T, \epsilon)$, respectively. For Scenario II, each point presents $\mu_T$ and the minimum value of $\tilde{m}^{sig}_{k}(\mu_T, \epsilon)$ taken over the 25 regression coefficients.

# 3 Results for example used to choose $M$ and $a$

In Section 6 of the main text, we discuss two regression examples. This section presents results from those models.

Table 1 and 2 display the p-values and signs associated with five independent queries of $\bar{T}^{t,\epsilon}$ for all 25 coefficients in the regression of income on $\mathbf{X}_{\boldsymbol{D}}$ in the CPS data. Table 1 is obtained by using Algorithms 1 and 2 from the main text and by fixing an upper bound for $L^{sig}_{t,\epsilon}(M, a, \epsilon)$ at 0.1, $\alpha = 0.05$, $\lambda_0 = 0.2$, $M = 25$, $a = 2$, and $\epsilon = 1.5$. Section 6 of the main text includes interpretations of the results displayed in Table 1.

Table 2 is obtained by using Algorithms 1 and 2 and by fixing an upper bound for $L^{sig}_{t,\epsilon}(M, a, \epsilon)$

at $0.2$, $\alpha = 0.05$, $\lambda_0 = 0.2$, $M = 100$, $a = 1$, and $\epsilon = 0.5$. As pointed out in Section 6 of the main text, we see different interpretations of the significance for 3 out of 25 coefficients—$\beta_3$, $\beta_8$, and $\beta_9$—in at least 3 out of the 5 queries. We have two conjectures about the reasons behind these differences. First, some of the categorical predictors have levels with a small number of observations. In such cases, we cannot provide an accurate estimate of the corresponding regression coefficients. For instance, in the first query, $\beta_3$, $\beta_8$, and $\beta_9$ are all coefficients associated with specific levels of education. For such levels, the average number of observations available to estimate $\beta_3$, $\beta_8$, and $\beta_9$ is around 5, 15, and 6, respectively. Second, assumption **A2** may not be reasonable for the CPS dataset when $M = 100$.

| | $T(\boldsymbol{D})$ | $\bar{T}^{RT,\epsilon}(\mathcal{P})$ Query 1 | Query 2 | Query 3 | Query 4 | Query 5 |
|---|---|---|---|---|---|---|
| $\beta_0$ | 0.000(+) | 0.000(+) | 0.000(+) | 0.000(+) | 0.000(+) | 0.000(+) |
| $\beta_1$ | 0.000(+) | 0.000(+) | 0.000(+) | 0.000(+) | 0.000(+) | 0.000(+) |
| $\beta_2$ | 0.000(-) | 0.000(-) | 0.000(-) | 0.000(-) | 0.000(-) | 0.000(-) |
| $\beta_3$ | 0.917(-) | 0.941(+) | 0.861(-) | 0.987(-) | 0.166(+) | 0.904(+) |
| $\beta_4$ | 0.271(+) | 0.794(-) | 0.430(+) | 0.225(+) | 0.337(+) | 0.180(+) |
| $\beta_5$ | 0.161(+) | 0.102(+) | 0.320(+) | 0.171(+) | 0.484(+) | 0.017(+) |
| $\beta_6$ | 0.054(+) | 0.033(+) | 0.657(+) | 0.102(+) | 0.154(+) | 0.007(+) |
| $\beta_7$ | 0.085(+) | 0.292(-) | 0.190(+) | 0.015(+) | 0.156(+) | 0.085(+) |
| $\beta_8$ | 0.020(+) | 0.050(+) | 0.049(+) | 0.182(+) | 0.008(+) | 0.078(+) |
| $\beta_9$ | 0.000(+) | 0.008(+) | 0.018(+) | 0.020(+) | 0.016(+) | 0.004(+) |
| $\beta_{10}$ | 0.000(+) | 0.000(+) | 0.000(+) | 0.000(+) | 0.000(+) | 0.000(+) |
| $\beta_{11}$ | 0.000(+) | 0.000(+) | 0.000(+) | 0.000(+) | 0.000(+) | 0.000(+) |
| $\beta_{12}$ | 0.000(+) | 0.000(+) | 0.000(+) | 0.000(+) | 0.000(+) | 0.000(+) |
| $\beta_{13}$ | 0.000(+) | 0.000(+) | 0.000(+) | 0.000(+) | 0.000(+) | 0.000(+) |
| $\beta_{14}$ | 0.000(+) | 0.000(+) | 0.000(+) | 0.000(+) | 0.000(+) | 0.000(+) |
| $\beta_{15}$ | 0.000(+) | 0.000(+) | 0.000(+) | 0.000(+) | 0.000(+) | 0.000(+) |
| $\beta_{16}$ | 0.000(+) | 0.000(+) | 0.000(+) | 0.000(+) | 0.000(+) | 0.000(+) |
| $\beta_{17}$ | 0.000(+) | 0.000(+) | 0.000(+) | 0.000(+) | 0.000(+) | 0.000(+) |
| $\beta_{18}$ | 0.461(-) | 0.990(-) | 0.267(-) | 0.272(-) | 0.679(-) | 0.458(-) |
| $\beta_{19}$ | 0.000(-) | 0.000(-) | 0.000(-) | 0.000(-) | 0.000(-) | 0.000(-) |
| $\beta_{20}$ | 0.000(-) | 0.000(-) | 0.000(-) | 0.000(-) | 0.000(-) | 0.000(-) |
| $\beta_{21}$ | 0.000(-) | 0.000(-) | 0.000(-) | 0.000(-) | 0.000(-) | 0.000(-) |
| $\beta_{22}$ | 0.000(-) | 0.000(-) | 0.000(-) | 0.000(-) | 0.000(-) | 0.000(-) |
| $\beta_{23}$ | 0.000(-) | 0.000(-) | 0.000(-) | 0.000(-) | 0.000(-) | 0.000(-) |
| $\beta_{24}$ | 0.000(-) | 0.000(-) | 0.000(-) | 0.000(-) | 0.000(-) | 0.000(-) |

Table 1: P-values and signs corresponding to the $25$ coefficients in the regression with the CPS dataset. P-values are rounded to the fourth decimal place. The first column shows the p-values and signs reported by the $t$-statistic. The last five columns show the p-values and signs obtained from five replications of $\bar{T}^{t,\epsilon}$, using $(M = 25, a = 2, \epsilon = 1.5)$. Each of the final five columns corresponds to a different query for the same coefficient.

| | $T(\boldsymbol{D})$ | $\bar{T}^{RT,\epsilon}(\mathcal{P})$ Query 1 | Query 2 | Query 3 | Query 4 | Query 5 |
|---|---|---|---|---|---|---|
| $\beta_0$ | 0.000(+) | 0.000(+) | 0.000(+) | 0.000(+) | 0.000(+) | 0.000(+) |
| $\beta_1$ | 0.000(+) | 0.000(+) | 0.000(+) | 0.000(+) | 0.000(+) | 0.000(+) |
| $\beta_2$ | 0.000(-) | 0.000(-) | 0.000(-) | 0.000(-) | 0.000(-) | 0.000(-) |
| $\beta_3$ | 0.917(-) | 0.009(-) | 0.021(-) | 0.033(-) | 0.208(-) | 0.234(-) |
| $\beta_4$ | 0.271(+) | 0.002(-) | 0.058(-) | 0.149(-) | 0.084(-) | 0.740(-) |
| $\beta_5$ | 0.161(+) | 0.223(-) | 0.113(-) | 0.294(-) | 0.056(-) | 0.526(+) |
| $\beta_6$ | 0.054(+) | 0.245(-) | 0.032(-) | 0.248(-) | 0.289(-) | 0.300(+) |
| $\beta_7$ | 0.085(+) | 0.000(-) | 0.307(-) | 0.644(+) | 0.143(-) | 0.804(+) |
| $\beta_8$ | 0.020(+) | 0.151(-) | 0.335(-) | 0.222(-) | 0.910(+) | 0.835(-) |
| $\beta_9$ | 0.000(+) | 0.508(-) | 0.949(-) | 0.703(-) | 0.998(+) | 0.496(+) |
| $\beta_{10}$ | 0.000(+) | 0.344(+) | 0.010(+) | 0.032(+) | 0.022(+) | 0.001(+) |
| $\beta_{11}$ | 0.000(+) | 0.068(+) | 0.001(+) | 0.000(+) | 0.001(+) | 0.000(+) |
| $\beta_{12}$ | 0.000(+) | 0.002(+) | 0.002(+) | 0.002(+) | 0.008(+) | 0.000(+) |
| $\beta_{13}$ | 0.000(+) | 0.003(+) | 0.000(+) | 0.000(+) | 0.000(+) | 0.000(+) |
| $\beta_{14}$ | 0.000(+) | 0.000(+) | 0.000(+) | 0.000(+) | 0.000(+) | 0.000(+) |
| $\beta_{15}$ | 0.000(+) | 0.000(+) | 0.000(+) | 0.000(+) | 0.000(+) | 0.000(+) |
| $\beta_{16}$ | 0.000(+) | 0.000(+) | 0.000(+) | 0.000(+) | 0.000(+) | 0.000(+) |
| $\beta_{17}$ | 0.000(+) | 0.000(+) | 0.000(+) | 0.000(+) | 0.000(+) | 0.000(+) |
| $\beta_{18}$ | 0.461(-) | 0.834(+) | 0.489(-) | 0.384(-) | 0.618(-) | 0.421(-) |
| $\beta_{19}$ | 0.000(-) | 0.000(-) | 0.000(-) | 0.000(-) | 0.000(-) | 0.000(-) |
| $\beta_{20}$ | 0.000(-) | 0.000(-) | 0.000(-) | 0.000(-) | 0.000(-) | 0.000(-) |
| $\beta_{21}$ | 0.000(-) | 0.000(-) | 0.000(-) | 0.000(-) | 0.000(-) | 0.000(-) |
| $\beta_{22}$ | 0.000(-) | 0.000(-) | 0.000(-) | 0.000(-) | 0.000(-) | 0.000(-) |
| $\beta_{23}$ | 0.000(-) | 0.000(-) | 0.000(-) | 0.000(-) | 0.000(-) | 0.000(-) |
| $\beta_{24}$ | 0.000(-) | 0.000(-) | 0.000(-) | 0.000(-) | 0.000(-) | 0.000(-) |

Table 2: P-values and signs corresponding to the $25$ coefficients in the regression with the CPS dataset. P-values are rounded to the fourth decimal place. The first column shows the p-values and signs reported by the $t$-statistic. The last five columns show the p-values and signs obtained from five replications of $\bar{T}^{t,\epsilon}$, using $(M = 100, a = 1, \epsilon = 0.5)$. Each of the final five columns corresponds to a different query for the same coefficient.
